# Supplementary material for: ApplicaAI at SemEval-2020 Task 11: On RoBERTa-CRF, Span CLS and Whether Self-Training Helps Them
Source: arXiv:2005.07934 source file (2020-09-05)
Supplement: Supplementary file 1 [file appendix.tex]

Appendix
